# Supplementary material for: Improving Autoregressive Training with Dynamic Oracles
Source: arXiv:2406.09393 source file (2024-06-13)
Supplement: Supplementary file 1 [file ner_appendix.tex]

% \begin{table*}[h]
%     \centering
%     \begin{tabular}{c c c c c}
    
    
%         \bf Dataset & \bf Model & \bf Configuration & \bf $F1_e$ (\%) & \bf $F1_p$ (\%)\\
%         \hline
%         \multicolumn{2}{c}{\textit{best published}}\\
%         CoNLL-2003(English) & FLAIR + CRF \cite{akbik-etal-2019-pooled} & & \bf 93.18 & \\
%         WNUT-2017 & FLAIR + CRF \cite{akbik-etal-2019-pooled} & & \bf 49.59 & \\
%         \hline
%         CoNLL-2003(English) & FLAIR + CRF & -  & 91.90 & 92.70 \\
%         CoNLL-2003(German) & FLAIR + CRF & -  & 86.80 & 87.90 \\
%         WNUT-2017 & FLAIR + CRF & -  & 46.99 & 48.97 \\
%         \midrule
%         CoNLL-2003(English) & FLAIR + RNN-LM & Teacher Forcing  & - & 91.50 \\
%         CoNLL-2003(English) & FLAIR + RNN-LM & Scheduled Sampling  & - & 92.72 \\
%         CoNLL-2003(English) & FLAIR + RNN-LM & Dynamic Oracle  & - & \bf93.08 \\
%         \midrule
%         WNUT-2017 & FLAIR + RNN-LM & Teacher Forcing  & - & 47.52 \\
%         WNUT-2017 & FLAIR + RNN-LM & Scheduled Sampling  & - & 48.91 \\
%         WNUT-2017 & FLAIR + RNN-LM & Dynamic Oracle  & - & \bf49.40 \\
%         \hline
%         \multicolumn{5}{c}{Here $F1_e$ and $F1_p$ are the exact match F1 and partial match F1 scores respectively.}
%     \end{tabular}
    
%     \caption{Results on NER}
%     \label{tab:NER_Results_appendix}
% \end{table*}

% \begin{table*}
%     \centering
%     \begin{tabular}{c c}
    
    
%         \bf Model & $F1_p$ (\%) \\
%         \hline
%         Char and Word LSTM + RNN-LM & 32.51 \\
%         BERT + RNN-LM & 44.23 \\
%         FLAIR + RNN-LM &  47.52\\
%         \hline
%     \end{tabular}
%     \caption{Results on WNUT-2017 with different embeddings}
%     \label{tab:WNUT-2017_Results}
% \end{table*}

% \begin{table*}
%     \centering
%     \begin{tabular}{c c}
    
    
%         \bf Model & $F1_p$ (\%) \\
%         \hline
%         Char and Word LSTM + RNN-LM & 79.91 \\
%         BERT + RNN-LM & 90.21 \\
%         FLAIR + RNN-LM& 91.50 \\
%         \hline
%     \end{tabular}
%     \caption{Results on CoNLL-2003(English) with different embeddings}
%     \label{tab:ner_appendix}
% \end{table*}
